# Supplementary material for: Scaling up Superconducting Quantum Computers with Cryogenic RF-photonics
Source: arXiv:2210.15756 source file (2022-10-27)
Supplement: Supplementary file 1 [file appendix.tex]

\appendix[Name]
\label{sec:appendix}

\begin{equation}
    \label{eq:samplers-gain}
    G_{S} = \frac{T_S}{\tau_S}
	\quad
    G_{R} = exp(\frac{T_R}{\tau_R}),
\end{equation}
